# Supplementary material for: Accurate and gate-efficient quantum ans\"atze for electronic states without adaptive optimisation
Source: arXiv:2312.09761 source file (2024-04-25)
Supplement: Supplementary file 2 [file SupplementaryMaterial.pdf]

# Symmetry-preserving and gate-efficient quantum circuits for quantum chemistry: Supplementary Material

Hugh G. A. Burton\*  
(Dated: December 15, 2023)

## Supplementary Methods

### Orbital optimisation

Orbital optimisation is essential to obtain smooth potential energy surfaces with truncated tUPS approximations. The molecular spatial orbitals  $|\phi_p\rangle$  are defined as a linear combination of  $N$  atomic orbitals  $|\chi_\mu\rangle$  as

$$|\phi_p\rangle = \sum_{\mu}^N |\chi_\mu\rangle C_{\cdot p}^{\mu}, \quad (1)$$

where we use the nonorthogonal tensor notation.<sup>(1)</sup> Assuming real orbitals, the coefficients  $C_{\cdot p}^{\mu}$  are orthogonalised to satisfy

$$\sum_{\mu\nu}^N C_{\cdot p}^{\mu} \langle \chi_\mu | \chi_\nu \rangle C_{\cdot q}^{\nu} = \delta_{pq}. \quad (2)$$

Variations in the orbital coefficients for the correlated wave function  $|\Psi\rangle$  can be parametrised using the exponential representation

$$|\Psi(s)\rangle = \exp\left(\sum_{m>n}^N s_{mn}(\hat{E}_{mn} - \hat{E}_{nm})\right) |\Psi\rangle, \quad (3)$$

where  $s$  is an  $N \times N$  anti-Hermitian matrix representing a step in the orbital space. The energy can be optimised with respect to the orbital coefficients by computing the gradient in this exponential representation, given by<sup>(2)</sup>

$$\left. \frac{\partial E}{\partial s_{mn}} \right|_{s=0} = 2(F_{mn} - F_{nm}), \quad (4)$$

where  $F_{mn}$  are matrix elements of the generalized Fock matrix and are defined as

$$F_{mn} = \sum_q^N D_{mq} h_{nq} + \sum_{qrs}^N \Gamma_{m qrs} g_{n qrs}. \quad (5)$$

Here,  $D_{pq} = \langle \Psi | \hat{E}_{pq} | \Psi \rangle$  and  $\Gamma_{pqrs} = \langle \Psi | \hat{e}_{pqrs} | \Psi \rangle$  are the one- and two-body reduced density matrices (RDMs) for the correlated wave function, respectively, and  $\hat{e}_{pqrs} = \hat{E}_{pq} \hat{E}_{rs} - \delta_{qr} \hat{E}_{ps}$ .<sup>(2)</sup> The one-electron and two-electron integrals are defined as  $h_{pq} = \langle \phi_p | \hat{h} | \phi_q \rangle$  and  $g_{pqrs} = (pq|rs)$ , respectively. The optimal step can then be implemented by re-computing the one- and two-electron integrals using the updated orbitals

$$\tilde{C} = C \exp(s). \quad (6)$$

Since this process only needs the one- and two-body RDMs, which are already measured to compute the energy on a quantum device, this orbital optimisation does not require any additional quantum resources.

In our current implementation, it is easier to include orbital optimisation using additional one-body unitary operations that are optimised as part of the VQE simulation. These unitary operations are applied after the standard tUPS circuit structure using repeating layers of nearest-neighbour spin-adapted one-body operators, as illustrated in Supplementary Figure 1. The number of layers required to implement any orbital transformation is determined by the number of unique orbital pairs  $\frac{1}{2}N(N-1)$ , which must match the number of one-body operators in the orbital transformation circuit. This circuit implementation has the same formal expressibility as transforming the molecular integrals. A similar approach is used for practical hardware experiments in Ref. (3).

### Molecular geometries

All nuclear coordinates are represented in angstroms. The bond distance for linear molecules is provided in the main text.

### Triangular $H_6$

Regular lattice with internuclear distance  $R(\text{H-H}) = 2.0 \text{ \AA}$ .

|   |        |        |        |
|---|--------|--------|--------|
| H | 0.0000 | 0.0000 | 0.0000 |
| H | 1.0000 | 1.7321 | 0.0000 |
| H | 2.0000 | 0.0000 | 0.0000 |
| H | 3.0000 | 1.7321 | 0.0000 |
| H | 4.0000 | 0.0000 | 0.0000 |
| H | 2.0000 | 3.4641 | 0.0000 |

### Benzene

Experimental structure obtained from the National Institute of Standards and Technology database.(4)

|   |         |         |        |
|---|---------|---------|--------|
| C | 1.3970  | 0.0000  | 0.0000 |
| C | 0.6985  | 1.2098  | 0.0000 |
| C | -0.6985 | 1.2098  | 0.0000 |
| C | -1.3970 | 0.0000  | 0.0000 |
| C | -0.6985 | -1.2098 | 0.0000 |
| C | 0.6985  | -1.2098 | 0.0000 |
| H | 2.4810  | 0.0000  | 0.0000 |
| H | 1.2405  | 2.1486  | 0.0000 |
| H | -1.2405 | 2.1486  | 0.0000 |
| H | -2.4810 | 0.0000  | 0.0000 |
| H | -1.2405 | -2.1486 | 0.0000 |
| H | 1.2405  | -2.1486 | 0.0000 |

### Water

- Variable bond length  $R(\text{O}-\text{H})$ .
- Fixed bond angle  $\angle\text{HOH} = 104.5^\circ$ .

### Be + $\text{H}_2$ insertion

A reaction pathway for the insertion of Be into  $\text{H}_2$  was constructed following the strategy of Refs. (5) and (6). Keeping the Be atom fixed, the H nuclear coordinates were varied as

|    |         |         |         |
|----|---------|---------|---------|
| Be | 0.00000 | 0.00000 | 0.00000 |
| H  | x       | -y      | 0.00000 |
| H  | x       | y       | 0.00000 |

using a grid defined as  $x_n = \frac{5.746708}{29}n$  and  $y_n = 1.31011 - 0.164183x_n$  for  $n = 0, 1, \dots, 29$ .

### Methylene

- Fixed bond length  $R(\text{C}-\text{H}) = 1.117 \text{ \AA}$ .
- Variable bond angle  $\angle\text{HCH}$ .

### Tetramethyleneethane

Structure obtained from *ab initio* geometry optimisation using restricted Hartree-Fock (STO-3G).

|   |               |               |               |
|---|---------------|---------------|---------------|
| C | 1.5191359612  | -1.2435560240 | 0.0000000000  |
| C | 0.7596227794  | 0.0236969349  | -0.0000000000 |
| C | -0.7595397676 | -0.0236632811 | -0.0000000000 |
| C | 1.4388758359  | 1.1618268649  | -0.0000000000 |
| C | -1.4388154450 | -1.1617811361 | -0.0000000000 |
| C | -1.5190270294 | 1.2436044768  | 0.0000000000  |
| H | 1.0485608349  | -2.2118574675 | 0.0000000000  |
| H | 2.5977393829  | -1.2079530524 | 0.0000000000  |
| H | 2.5193775927  | 1.1619199006  | -0.0000000000 |
| H | 0.9765986939  | 2.1353834069  | -0.0000000000 |
| H | -0.9765601118 | -2.1353473098 | -0.0000000000 |
| H | -2.5193178879 | -1.1618520565 | -0.0000000000 |
| H | -2.5976311650 | 1.2080244996  | 0.0000000000  |
| H | -1.0484295180 | 2.2118956990  | 0.0000000000  |

## Supplementary Discussion

### Relating fermionic operators to Given's rotations

The action of  $\exp(\theta\hat{\kappa}_{pq}^{(1)})$  and  $\exp(\theta\hat{\kappa}_{pq}^{(2)})$  for many-electron systems can be understood by considering how these operators transform many-body Slater determinants. For a given  $(p, q)$  pair, we can group determinants according to their occupation of the orbitals  $\phi_p$  and  $\phi_q$ . In what follows, an arbitrary determinant is denoted  $|k_p k_q k_{\bar{q}} k_{\bar{p}}; \mathbf{k}'\rangle$ , where  $k_p$  ( $k_{\bar{p}}$ ) are the occupation numbers of the high (low) spin orbital corresponding to  $\phi_p$ , and  $\mathbf{k}'$  is the occupation vector for orbitals excluding  $p$  and  $q$ . Since neither  $\hat{\kappa}_{pq}^{(1)}$  or  $\hat{\kappa}_{pq}^{(2)}$  can change the occupation of any orbital except  $\phi_p$  or  $\phi_q$ , matrix representations for each  $\mathbf{k}'$  can be expressed as

$$\hat{\kappa}_{pq}^{(1)} = \begin{pmatrix} 0 & & & & & \\ & 0 & -1 & & & \\ & 1 & 0 & & & \\ & & & 0 & -1 & \\ & & & 1 & 0 & \\ & & & & & 0 \\ & & & & 0 & -1 & -1 & 0 \\ & & & & 1 & 0 & 0 & -1 \\ & & & & 1 & 0 & 0 & -1 \\ & & & & 0 & 1 & 1 & 0 \\ & & & & & & & 0 \\ & & & & & & 0 & -1 \\ & & & & & & 1 & 0 \\ & & & & & & & 0 & -1 \\ & & & & & & & 1 & 0 \\ & & & & & & & & 0 \end{pmatrix}, \quad \hat{\kappa}_{pq}^{(2)} = \begin{pmatrix} 0 & & & & & \\ & 0 & & & & \\ & & 0 & & & \\ & & & 0 & & \\ & & & & 0 & \\ & & & & & 0 \\ & & & & 0 & 0 & 0 & -2 \\ & & & & 0 & 0 & 0 & 0 \\ & & & & 0 & 0 & 0 & 0 \\ & & & & 0 & 0 & 0 & 0 \\ & & & & 2 & 0 & 0 & 0 \\ & & & & & & & 0 \\ & & & & & & 0 & & 0 \\ & & & & & & & 0 & & 0 \\ & & & & & & & & 0 & & 0 \\ & & & & & & & & & 0 & \\ & & & & & & & & & & 0 \end{pmatrix}$$

(7)

where the occupation numbers  $|k_q k_p k_{\bar{q}} k_{\bar{p}}\rangle$  are ordered as

$$\{|0000\rangle, |1000\rangle, |0100\rangle, |0010\rangle, |0001\rangle, |1100\rangle, |1010\rangle, |1001\rangle, |0110\rangle, |0101\rangle, |0011\rangle, |1110\rangle, |1101\rangle, |1011\rangle, |0111\rangle, |1111\rangle\} \quad (8)$$

and the remaining zeros have been omitted to highlight the block diagonal structure. These matrix representations reveal the relationship of  $\exp(\theta \hat{\kappa}_{pq}^{(1)})$  and  $\exp(\theta \hat{\kappa}_{pq}^{(2)})$  to Given's rotations.(7) In particular, since the high- and low-spin one-body operators commute (i.e.  $[\hat{\tau}_{pq}, \hat{\tau}_{\bar{p}\bar{q}}] = 0$  where  $\hat{\tau}_{pq} = \hat{p}^\dagger \hat{q} - \hat{q}^\dagger \hat{p}$ ), the one-body exponential operator corresponds to the product of two Given's rotations as  $\exp(\theta \hat{\kappa}_{pq}^{(1)}) = \exp(\theta \hat{\tau}_{pq}) \exp(\theta \hat{\tau}_{\bar{p}\bar{q}})$ . The Given's rotation  $\exp(\theta \hat{\tau}_{pq})$  only affects the occupancies of the high-spin orbitals corresponding to  $\phi_p$  and  $\phi_q$ , and similarly for the low-spin counterpart  $\exp(\theta \hat{\tau}_{\bar{p}\bar{q}})$ . Analogously, the paired two-body exponential operator  $\exp(\theta \hat{\kappa}_{pq}^{(2)})$  corresponds to a Given's rotation between the determinants with occupancies  $|k_q k_p k_{\bar{q}} k_{\bar{p}}\rangle$  corresponding to  $|1010\rangle$  and  $|0101\rangle$ .(7) Through this relationship, the tUPS *ansatz* embraces the natural capabilities of qubit rotations in quantum computation, providing a bridge between physically-motivated and hardware-efficient approximations.

### Universality of the $t$ UPS wave function

Previously, the universality of UPS wave functions constructed from spin-adapted one-body and paired two-body operators was derived by showing that all many-body fermionic operators can be represented as nested commutator expansions of  $\hat{\kappa}_{pq}^{(1)}$  and  $\hat{\kappa}_{pq}^{(2)}$ .<sup>(8, 9)</sup> The universality of the tUPS circuit structure can be shown by representing  $\hat{\kappa}_{pq}^{(1)}$  and  $\hat{\kappa}_{pq}^{(2)}$  as nested commutators containing only operators that act between sequential spatial orbitals, i.e.  $\hat{\kappa}_{p,p\pm 1}^{(1)}$  and  $\hat{\kappa}_{p,p\pm 1}^{(2)}$ . These operators are shown to be sufficient by representing the non-sequential spin-adapted one-body and paired two-body operators as

$$\hat{\kappa}_{p,p+2}^{(1)} = [\hat{\kappa}_{p,p+1}^{(1)}, \hat{\kappa}_{p+1,p+2}^{(1)}], \quad (9a)$$

$$\hat{\kappa}_{p,p+2}^{(2)} = \frac{1}{2} \left[ \hat{\kappa}_{p,p+1}^{(1)}, [\hat{\kappa}_{p,p+1}^{(1)}, \hat{\kappa}_{p+1,p+2}^{(2)}] \right] + \hat{\kappa}_{p+1,p+2}^{(2)}. \quad (9b)$$

Through these expressions, the exponential operators can be implemented using the identities  $e^{\hat{A}+\hat{B}} = \lim_{n \rightarrow \infty} (e^{\hat{A}} e^{\hat{B}})^n$  and  $e^{[\hat{A}, \hat{B}]} = \lim_{n \rightarrow \infty} (e^{\hat{A}/\sqrt{n}} e^{\hat{B}/\sqrt{n}} e^{-\hat{A}/\sqrt{n}} e^{-\hat{B}/\sqrt{n}})^n$ .

Eq. (9a) can be derived using the standard commutator rule  $[\hat{E}_{pq}, \hat{E}_{rs}] = \delta_{qr}\hat{E}_{ps} - \delta_{ps}\hat{E}_{rq}$  as

$$\begin{aligned} [\hat{\kappa}_{p,p+1}^{(1)}, \hat{\kappa}_{p+1,p+2}^{(1)}] &= [\hat{E}_{p,p+1} - \hat{E}_{p+1,p}, \hat{E}_{p+1,p+2} - \hat{E}_{p+2,p+1}] \\ &= [\hat{E}_{p,p+1}, \hat{E}_{p+1,p+2}] - [\hat{E}_{p+1,p}, \hat{E}_{p+1,p+2}] - [\hat{E}_{p,p+1}, \hat{E}_{p+2,p+1}] + [\hat{E}_{p+1,p}, \hat{E}_{p+2,p+1}] \\ &= \hat{E}_{p,p+2} - \hat{E}_{p+2,p} \\ &= \hat{\kappa}_{p,p+2}^{(1)}. \end{aligned} \quad (10)$$

Similarly, noting that  $\hat{\kappa}_{pq}^{(2)} = \hat{e}_{pqpq} - \hat{e}_{qpqp}$ , where  $\hat{e}_{pqrs} = \hat{E}_{pq}\hat{E}_{rs} - \delta_{qr}\hat{E}_{ps}$ , we can use the commutator identity(2)  $[\hat{E}_{mn}, \hat{e}_{pqrs}] = \delta_{pn}\hat{e}_{mqrs} + \delta_{rn}\hat{e}_{pqms} - \delta_{mq}\hat{e}_{pnrs} - \delta_{ms}\hat{e}_{pqrn}$  to expand the nested commutator in Eq. (9b) as

$$\begin{aligned} [\hat{\kappa}_{p,p+1}^{(1)}, [\hat{\kappa}_{p,p+1}^{(1)}, \hat{\kappa}_{p+1,p+2}^{(2)}]] &= [\hat{E}_{p,p+1} - \hat{E}_{p+1,p}, [\hat{E}_{p,p+1} - \hat{E}_{p+1,p}, \hat{e}_{p+1,p+2,p+1,p+2} - \hat{e}_{p+2,p+1,p+2,p+1}]] \\ &= [\hat{E}_{p,p+1} - \hat{E}_{p+1,p}, \hat{e}_{p,p+2,p+1,p+2} + \hat{e}_{p+1,p+2,p,p+2} - \hat{e}_{p+2,p,p+2,p+1} + \hat{e}_{p+2,p+1,p+2,p}] \\ &= 2(\hat{e}_{p,p+2,p,p+2} - \hat{e}_{p+2,p,p+2,p}) - 2(\hat{e}_{p+1,p+2,p+1,p+2} - \hat{e}_{p+2,p+1,p+2,p+1}) \\ &= 2\hat{\kappa}_{p,p+2}^{(2)} - 2\hat{\kappa}_{p+1,p+2}^{(2)} \end{aligned} \quad (11)$$

from which the full expression in Eq. (9b) can be obtained.

Here, we have shown that arbitrary spin-adapted one-body and paired two-body operators can be expressed purely as a sum of operators acting between sequential spatial orbitals and their commutators. Therefore, the product of exponential operators in the tUPS *ansatz* with an increasing number of layers will eventually be able to parametrise any exponential operation for the Lie algebra of many-body excitations, as indicated through successive applications of the Baker–Campbell–Hausdorff expansion  $e^{\hat{A}}e^{\hat{B}} = e^{\hat{A}+\hat{B}+\frac{1}{2}[\hat{A},\hat{B}]+\dots}$ .(10) Consequently, exact wave functions within a finite basis set can be obtained with a sufficient number of layers, which we expect to be finite in practice.

### Parameter shift rule for tUPS gradients

Computing partial derivatives of the energy with respect to the tUPS wave function parameters is essential for practical VQE simulations and gradients. Since the energy is periodic with respect to the *ansatz* parameters, a parameter-shift rule can be used to compute analytic gradients using the same variational circuit architecture as the energy computation.(11) The required parameter-shift rule can be deduced by examining the eigenvalue structure of  $\hat{\kappa}_{pq}^{(1)}$  and  $\hat{\kappa}_{pq}^{(2)}$ . First, we consider partial derivatives with respect to a parameter defining an exponential spin-adapted one-body operator  $\exp(\theta_1 \hat{\kappa}_{pq}^{(1)})$ . From Eq. (7), the unique eigenvalues of  $\hat{\kappa}_{pq}^{(1)}$  are 0,  $\pm 1i$ , and  $\pm 2i$ . Therefore, the exact partial derivative can be computed using a generalised four-point parameter shift rule(12)

$$\nabla_{\theta_1} E = \left[ E\left(\theta_1 + \frac{\pi}{4}\right) - E\left(\theta_1 - \frac{\pi}{4}\right) \right] + \left( \frac{1 - \sqrt{2}}{2} \right) \left[ E\left(\theta_1 + \frac{\pi}{2}\right) - E\left(\theta_1 - \frac{\pi}{2}\right) \right], \quad (12)$$

as derived in Ref. (13). Similarly, the eigenvalues of  $\hat{\kappa}_{pq}^{(2)}$  are 0, and  $\pm 2i$ , and thus the exact partial derivative for an exponential paired two-body operator  $\exp(\theta_2 \hat{\kappa}_{pq}^{(2)})$  can be computed with the two-point parameter shift rule

$$\nabla_{\theta_2} E = E\left(\theta_2 + \frac{\pi}{4}\right) - E\left(\theta_2 - \frac{\pi}{4}\right). \quad (13)$$

### Connection to perfect pairing theory

Perfect pairing (PP) theory is a well-established classical valence bond approximation for molecular systems.(14–18) Starting from a closed-shell Slater determinant, the PP wave function is constructed by assigning a unique virtual orbital  $\phi_{i^*}$  to each occupied spatial orbital  $\phi_i$  and considering all excitations between each occupied-virtual orbital pair. Arbitrary mixing between the singlet states for each occupied-virtual orbital pair can be parametrised with two rotation angles  $(x_i, y_i)$  and the total wave function for  $n$  electron pairs can then be expressed as the anti-symmetrised product

$$|\Psi_{\text{PP}}\rangle = \hat{\mathcal{A}} \prod_{i=1}^n \left( \cos x_i \cos y_i \phi_i \phi_{\bar{i}} + \frac{\sin x_i \cos y_i}{\sqrt{2}} (\phi_i \phi_{\bar{i}^*} + \phi_{i^*} \phi_{\bar{i}}) + \cos y_i \phi_{i^*} \phi_{\bar{i}^*} \right). \quad (14)$$

This wave function corresponds to a product of non-interacting singlet-coupled electron pairs and has been instrumental in developing our understanding of molecular bonding.(17, 19) It can accurately describe the dissociation of a single bond, but requires additional improvements to capture strongly interacting pairs of spin-coupled electrons.(20, 21) The equivalence between

the first half-layer of the pp-tUPS *ansatz* (see Fig. 2) and the PP wave function arises because the operators  $\hat{U}_{2p,2p-1}^{(1)}$  can exactly solve each (2e, 2o) sub-problem, giving a direct product of exact two-orbital sub-problems analogous to Eq. (14).

### Supplementary Figures

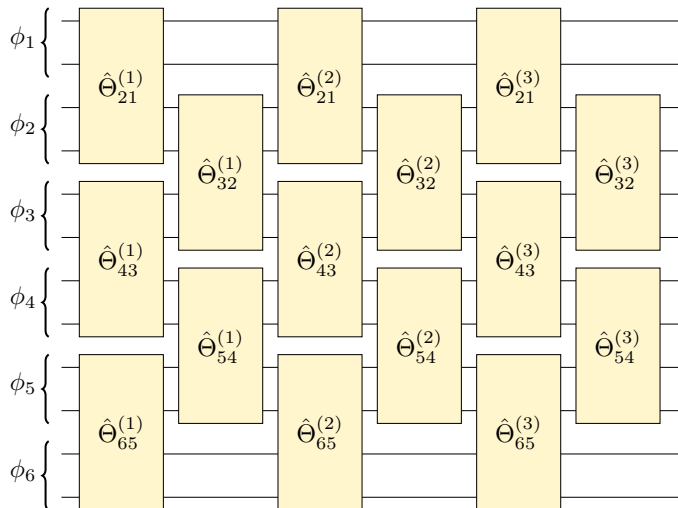

Supplementary Figure 1: Structure of the circuit applied to parametrise orbital optimisation in the current VQE simulations. This circuit is applied after the standard tUPS *ansatz* construction. The unitary operations  $\hat{\Theta}_{p+1,p}^{(m)} = \exp(\theta_{p+1,p}^{(m)} \hat{\kappa}_{p+1,p}^{(1)})$  are exponential spin-adapted one-body operators between nearest-neighbour spatial orbitals, with a unique parameter for each repetition  $m$ . The total number of operators matches the dimensionality of the orbital rotation space, e.g., 15 for 6 spatial orbitals.

### Supplementary Tables

Supplementary Table I: The continuous optimisation of the tUPS, oo-tUPS, and pp-tUPS *ansätze* was performed using basin-hopping parallel tempering (BHPT) to efficiently search for the global minimum, as summarised for VQE simulations in Ref. (9). This BHPT scheme included eight replica basin-hopping calculations with temperatures distributed exponentially between  $0.0001 E_h$  and  $0.01 E_h$ , and exchange between replicas was attempted with a mean frequency of 10 steps. On each basin-hopping step, the L-BFGS optimisation was converged to a root-mean-square gradient value below  $10^{-6} E_h$  and a maximum of 2000 steps. The number of frozen orbitals, the Hilbert space size, and the total number of basin-hopping steps per temperature replica is tabulated for each molecule.

| Molecule                  | Frozen core | Frozen virtuals | Hilbert Space Size | Basin-Hopping Steps per replica |
|---------------------------|-------------|-----------------|--------------------|---------------------------------|
| Linear H <sub>6</sub>     | 0           | 0               | 400                | 1000                            |
| Triangular H <sub>6</sub> | 0           | 0               | 400                | 1000                            |
| LiH                       | 0           | 0               | 225                | 1000                            |
| Benzene                   | 18          | 12              | 400                | 1000                            |
| H <sub>2</sub> O          | 0           | 0               | 441                | 1000                            |
| N <sub>2</sub>            | 4           | 0               | 400                | 1000                            |
| BeH <sub>2</sub>          | 0           | 0               | 1225               | 250                             |
| CH <sub>2</sub>           | 0           | 0               | 1225               | 1000                            |
| Tetramethyleneethane      | 19          | 13              | 400                | 1000                            |

### Supplementary References

\* [hgaburton@gmail.com](mailto:hgaburton@gmail.com)

- [1] M. Head-Gordon, P. E. Maslen, C. A. White, A tensor formulation of many-electron theory in a nonorthogonal single-particle basis, *J. Chem. Phys.* **108**, 616 (1998).
- [2] T. Helgaker, P. Jørgensen, J. Olsen, *Molecular Electronic-Structure Theory* (John Wiley & Sons, 2000).
- [3] G. A. Quantum, *et al.*, Hartree-Fock on a superconducting qubit quantum computer, *Science* **369**, 1084 (2020).

- [4] Computational chemistry comparison and benchmark database, <https://cccbdb.nist.gov/expgeom2x.asp>. Accessed: 2022-10-03.
- [5] F. A. Evangelista, Alternative single-reference coupled cluster approaches for multireference problems: The simpler the better, *J. Chem. Phys.* **134**, 224102 (2011).
- [6] I. Magoulas, F. A. Evangelista, CNOT-Efficient Circuits for Arbitrary Rank Many-Body Fermionic and Qubit Excitations, *J. Chem. Theory Comput.* **19**, 822 (2023).
- [7] J. M. Arrazola, *et al.*, Universal quantum circuits for quantum chemistry, *Quantum* **6**, 742 (2022).
- [8] F. A. Evangelista, G. K.-L. Chan, G. E. Scuseria, Exact parameterization of fermionic functions via unitary coupled cluster theory, *J. Chem. Phys.* **151**, 244122 (2019).
- [9] H. G. A. Burton, D. Marti-Dafcik, D. P. Tew, D. J. Wales, Exact electronic states with shallow quantum circuits from global optimisation, *npj Quantum Inf.* **9**, 75 (2023).
- [10] R. Gilmore, *Lie Groups, Physics, and Geometry: An Introduction for Physicists, Engineers, and Chemists* (Dover Publications Inc., 2008), first edn.
- [11] K. Mitarai, M. Negoro, M. Kitagawa, K. Fujii, Quantum circuit learning, *Phys. Rev. A* **98**, 032309 (2018).
- [12] D. Wierichs, J. Izaac, C. Wang, C. Y.-Y. Lin, General parameter-shift rules for quantum gradients, *Quantum* **6**, 677 (2022).
- [13] G.-L. R. Anselmetti, D. Wierichs, C. Gogolin, R. M. Parrish, Local, expressive, quantum-number-preserving VQE ansätze for fermionic systems, *New J. Phys.* **23**, 113010 (2021).
- [14] K. V. Lawler, D. W. Small, M. Head-Gordon, Orbitals That Are Unrestricted in Active Pairs for Generalized Valence Bond Coupled Cluster Methods, *J. Phys. Chem. A* **114**, 2930 (2010).
- [15] G. J. O. Beran, B. Austin, A. Sodt, M. Head-Gordon, Unrestricted Perfect Pairing: The Simplest Wave-Function-Based Model Chemistry beyond Mean Field, *J. Phys. Chem. A* **109**, 9183 (2005).
- [16] T. Van Voorhis, M. Head-Gordon, A nonorthogonal approach to perfect pairing, *J. Chem. Phys.* **112**, 5633 (2000).
- [17] A. C. Hurley, J. E. Lennard-Jones, J. A. Pople, The molecular orbital theory of chemical valency XVI. A theory of paired-electrons in polyatomic molecules, *Proc. Royal Soc. A* **220**, 446 (1953).
- [18] S. Lehtola, J. Parkhill, M. Head-Gordon, Orbital optimisation in the perfect pairing hierarchy: applications to full-valence calculations on linear polyacenes, *Mol. Phys.* **116**, 547 (2018).
- [19] C. E. Dykstra, Perfect pairing valence bond generalization of self-consistent electron pair theory, *J. Chem. Phys.* **72**, 2928 (1980).
- [20] J. A. Parkhill, M. Head-Gordon, A tractable and accurate electronic structure method for static correlations: The perfect hexuples model, *J. Chem. Phys.* **133**, 024103 (2010).
- [21] D. W. Small, M. Head-Gordon, Tractable spin-pure methods for bond breaking: Local many-electron spin-vector sets and an approximate valence bond model, *J. Chem. Phys.* **130**, 084103 (2009).
